# Supplementary material for: Credit Default Swaps Drawup Networks: Too Tied To Be Stable?
Source: arXiv:1205.0976 source file (2012-05-04)
Supplement: Supplementary file 1 [file SI_CDSPaper_2012_03_22.pdf]

# Supplementary Material
# Credit Default Swaps Drawup Networks: Too Tied To Be Stable?

**Rahul Kaushik and Stefano Battiston**
Chair of Systems Design, ETH Zurich, Switzerland
rkaushik@ethz.ch, sbattiston@ethz.ch

# 1 Motivations

*Credit Default Swap's* (CDS) are important for purposes of hedging, diversification and in some instances participating in markets that would be otherwise inaccessible to a subset of the market participants.

Even though CDS's are valuable to mitigate risks, they also tend to add to the fragility of a system. In the absence of a proper regulatory framework, CDS's can be used to accelerate the fragility of a firm, as was the case with *Lehman Brothers* in the financial crisis of 2008.

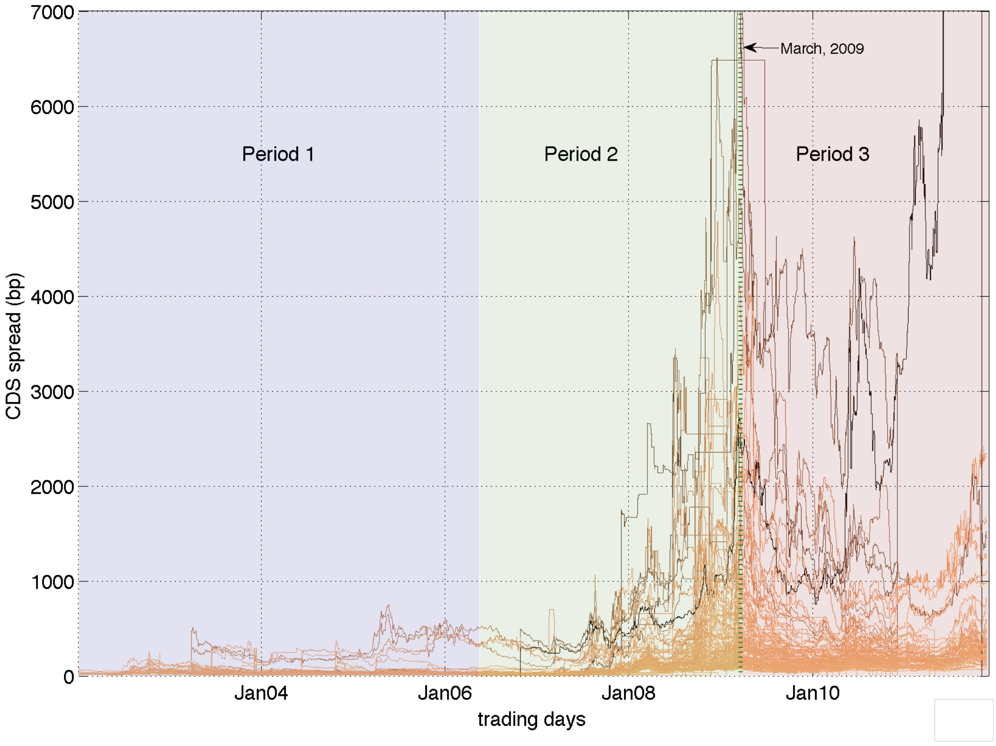


Figure 1: **Time series of credit default swaps throughout the credit crisis**. A plot of the CDS spread time series covering the financial crisis of 2008. The data ranges from January 2002 to December 2011. We can observe three market phases. Most CDS spreads peak around March 2009.

## 2 Background Information on CDS

A CDS is a bilateral Over the Counter (OTC) derivative. It is analogous to an insurance instrument. A CDS contract has three legs, i.e., there are three entities that formulate a CDS contract. The three parties involved in a typical CDS contract are the buyer, seller and reference entity. The buyer of a CDS contract purchases protection on the reference entity from the seller for fixed periodic payments, also called premiums. Roughly speaking, Fixed payments are determined by multiplying the premium (quoted in percentages) with the total value of protection sought, say $N$. It is not required that a buyer of a CDS contract have a credit exposure to a reference on which it is buying a CDS contract. Analogously, it is equivalent to saying that one can buy an insurance on one's neighbours house.

In the event that the reference entity defaults on its debt to its investors, the buyer receives a one time payment from the seller, hence the name *Credit Default Swap*. CDS's can be one of the following types: single name, Index and Basket CDS. As the names might suggest, single name CDS are on a single entity, sovereign or otherwise. Index CDS's are issued on constituents of an index with equal weights being assigned to each of the constituents. Basket CDS's can have more than one reference entity, in fact a basket of entities constitute a set of reference entities.

In the case of basket CDS's there are three further classifications, namely first-to-default CDS, full-basket CDS, untranched basket and a tranched basket, or Collateralised Debt Obligations (CDO). In addition, CDS contracts are negotiated privately and are bilateral in nature.

Like a swap agreement there is no initial payment that is needed to enter into a CDS contract. Unlike a corporate bond, a CDS contract enables a participant to go short in the credit of a reference entity. Also, one can enter into a CDS contract even if a corporate bond of some pre-specified maturity is not available.

The popularity of the CDS market can be seem from the growth of such products. International Swap and Derivatives Association (ISDA) statistics show that by the end of 2003, the notional amounts outstanding in the CDS markets stood at \$3.58 trillion dollars. Compared to the year 2000, in the year 2003 the CDS markets gained 1.4% percent of the entire swap market. The popularity of CDS contracts declined in the years 2009 and 2010. This was a fallout for the financial crisis of 2008. From figure 1 (main paper), we can see that the CDS spreads were reflecting such movements in the market. The embedded relationships that lie within a CDS contract remain opaque to the general public due to the fact that they are not only privately negotiated; but, also because information on such contracts exposes the financial institutions to corporate attacks. In addition, even if a comprehensive dataset were available, the lack of transparency with regards to ownerships leads to different level of complexity, see Battiston et al. (2010). To further elaborate on dependence structures that can arise in the CDS markets we present a small discussion on CDS configurations.

# 3 CDS Configurations

In order to understand what co-dependencies can arise between CDS market participants, we have first constructed a representative set of configurations of connections that market participants can develop over time in a given scenario. The motivation for such a breakdown is to account for preferences of market participants that emerge given a regulatory framework, or any other market factors. For example, banks, keeping in line with their mandate, tend to be broker dealers. This implies that they are both a buyer and seller of insurance contracts. A pension fund for example, typically tends to purchase protection to hedge its portfolio from loss due to its exposure to another entity; however, it tends to limit its transactional activity to being long on such instruments. Building upon the intuition we gather from the arguments above we can then divide dependence scenarios into three classes:

1. The set of buyers, sellers and reference entities are unique and non-overlapping sets.
2. The set of one of buyers, sellers, or reference entities overlaps with another, but not both
3. Each of the buyer can be a seller or a reference entity, or both

We have studied the dependence in each of these classes. Since the exact and detailed information on each of the CDS contracts is unavailable. If we restrict ourselves to the market dynamics, where each of the buyers, sellers and reference entities are non-separable, third class 3, we are able to explain co-movements in CDS spreads of two reference entities; since, CDS spread data, by construction,reflects the financial health of reference entities.

We now elaborate on each of the configurations stated above. The CDS contracts can be bought and sold for speculative purposes. This means that a market participant can purchase a CDS contract on another firm in the absence of any credit relationship between the two market participants. In this study we limit ourselves to analysing dependence structures do not arise out of speculative. In other words, we analyse dependence structures when market participants have pre-existing credit relationships and trade CDS contracts to hedge their respective risks. In addition, it is important to remember that in the event of a default, the CDS buyer is paid approximately 60% of the notional that is embedded in the notional of the CDS contract. This means that, if firm A is exposed to B in the amount of $100 and purchases protection from C on B. In the event that B defaults, then C would pay $60 to A.

The kind of dependence structure that emerges within the CDS market framework would largely depend on the intersection of set of buyers, sellers and reference entities. Thus, we explore the dependence structures that emerge when we study the permutations of possible intersecting sets of buyers, sellers and reference entities. It is important to remember here that the set of configurations that we present herein are in no way an exhaustive set of configurations. We

merely present some specific configurations that provide a good intuition on the dependencies that can emerge due to trading of CDS contracts. We encourage the reader to further explore these configurations.

## 3.1 Buyers, Sellers and Reference entities are unique:

We start with the first set configurations that emerge when we keep the set of buyers, sellers and reference entities as unique, i.e., the set of buyers, sellers and reference entities do not have have any common market participants (see 3.1).

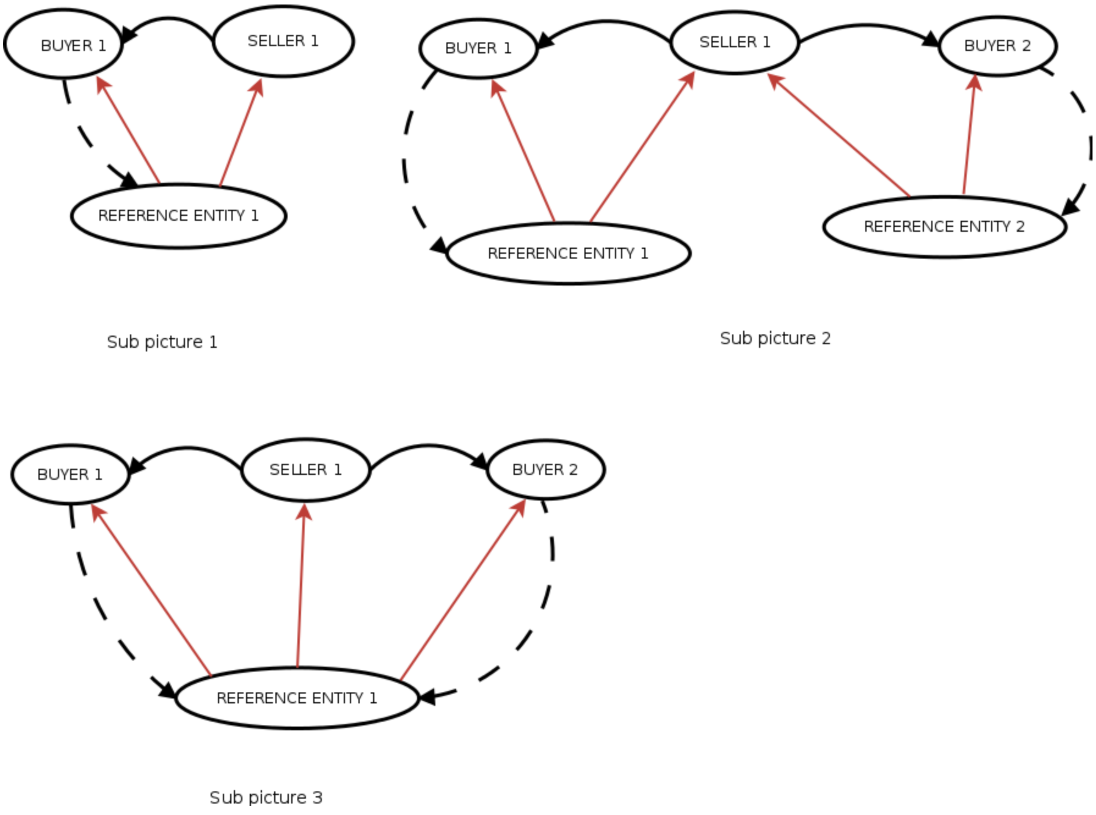


Figure 2: **Networks that exist when the buyers, sellers and reference entities are all unique**. The solid arrow moves from the seller of a CDS contract to the buyer. The dotted arrow refers to the reference entity underlying the CDS contract. The red arrows represent the direction of impact in the event of a default of the node from which the arrow emerges

We present three pictures for three scenarios (not exhaustive) for this particular market configuration, figure 3.1. Here the picture denotes some simple networks that may exist between

financial entities with regards to a single CDS transaction. The solid arrow moves from the seller of a CDS contract to the buyer. The dotted arrow refers to the reference entity underlying the CDS contract. The red arrows represent the direction of impact in the event the node, from which the arrow emerges, defaults.

**Scenario 1: Sub picture 1**
In this scenario we limit each CDS transaction limited to a unique seller, buyer, and reference entity. We find that in the event that reference entity 1 defaults, then both seller 1, and buyer 1 would experience an increase in their fragility. Buyer 1 would have lost 40% of its investment in reference entity 1. And, seller 1 would be liable for 60% of buyer 1's exposure to reference entity 1. In this case we find that the bulk of the burden due to default lands on the shoulders of the sellers.

**Scenario 2: Sub picture 2**
In this scenario we impose that a seller can have more than one buyer and more than one reference entity for protection. In the event, that either of the reference entities default, the corresponding buyer and the seller would experience an increase an fragility. Interestingly, if reference entity 1 defaults, then the fragility of buyer 2 would also get affected. Since, seller 1 is the insuring agent for reference entities 1 & 2. Thus, a default in either of the reference entities would make the seller more fragile. This in turn would lead to fragility of its other counterparties. Thus, we find that in this scenario that the fragility of reference entity 2 can also contribute to the fragility buyer 1 as they are both connected to the same seller.

**Scenario 3: Sub picture 3**
In this scenario we investigate a dependence structure whence a seller is liable to two buyers based on the same reference entity. If reference entity 1 defaults then all the market participants experience an increase in fragility, seller 1 being the agent that would suffer the most.

In the first part of the picture (Sub-picture 1), we see that in the event that reference entity 1 defaults, seller 1 is liable to buyer 1 to amount of the contingent claim. In sub-picture 2, we see that seller 1 has sold CDS contracts to buyer 1 and 2, on reference entities 1 and 2 respectively. It is clear from this picture that, in the unlikely event that either/both reference entities 1, 2 default; seller 1 is liable for contingent claims against it. In sub-picture 3, seller 1 is liable for reference entity 1's default to buyer 1 and 2.

In this set of configurations we find that the burden, in the event of a default, is almost entirely upon the sellers of the CDS contracts. However, we have seen from the financial crisis of 2008, that there were many institutions that were not necessarily sellers of CDS contracts, but also mainly buyers. A varied set of market participants were adversely affected from the fallout in the CDS market. Thus, we extend our argument to the set of CDS configurations, where the set of buyers and sellers have a non-trivial overlap.

## 3.2 Buyers-Sellers non-separable

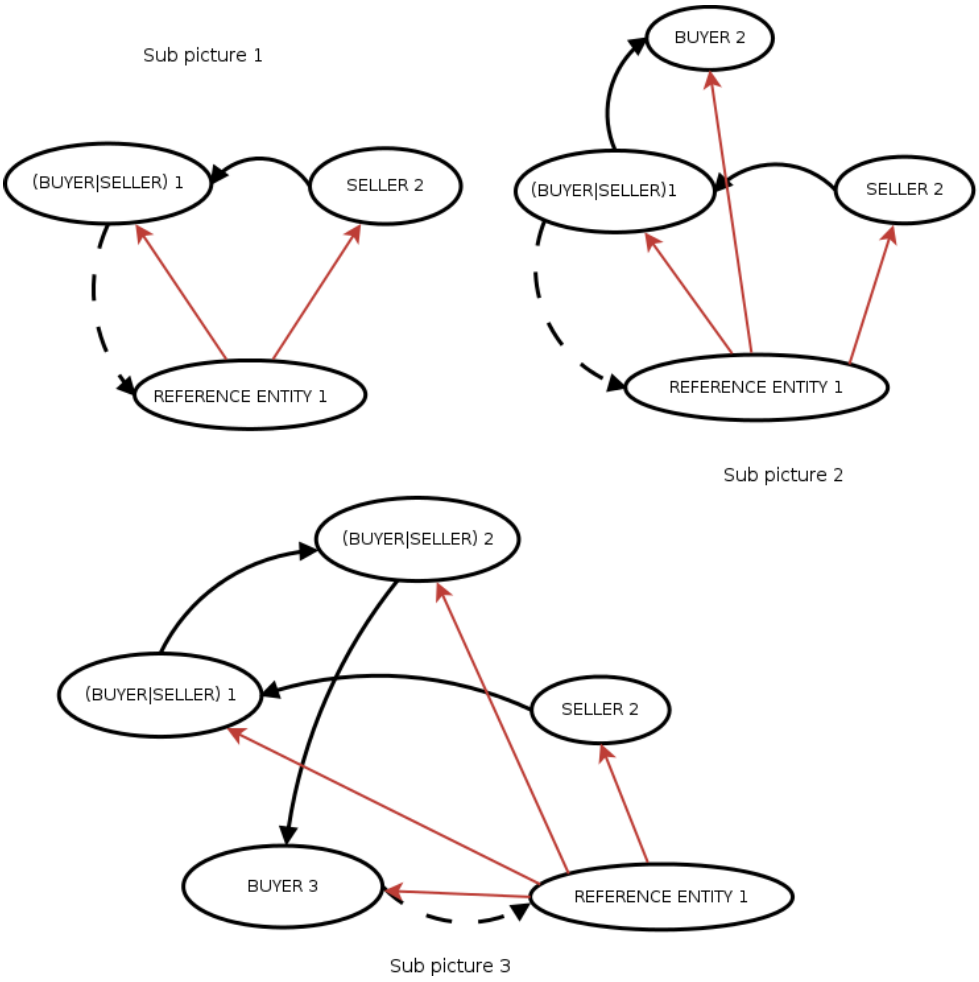


Figure 3: **Networks that exist when the buyers and sellers are the same but different from reference entities**. The solid arrow moves from the seller of a CDS contract to the buyer. The dotted arrow refers to the reference entity underlying the CDS contract. The red arrows represent the direction of impact in the event of a default of the node from which the arrow emerges

Consider sub picture 1 from figure 3, the arrows and lines represent the same relationships as before. From figure 3 (Sub picture 1) we see that $(Buyer|Seller)_1$ has bought a CDS contract from $Seller_2$, where the reference entity involved in the transaction is $Reference_1$.

**Scenario 1: Sub-picture 1**

The dependence structure that arises due to such a configuration is very similar to the dependence

that arises from scenario 1 whence the buyers, sellers, and reference entities are unique. Consider now the case that $Buyer_2$ is also a seller, (figure 3 Sub picture 3). In this case, the fragility of *Seller 2* affects the fragility of $(Buyer|Seller)_1$, which in turn would affects the others. Given the fragility of *Seller 2*, a default of $Reference_1$ would, more or less, make the entire system fragile.

**Scenario 2: Sub-picture 2** In this case we find that the default of reference entity 1 would affect seller 2, buyer 2, and buyer|seller 1.

**Scenario 3: Sub-picture 3** In this scenario we see that a default of reference entity 1 would affect all the market participants. However, it is worth noting here that buyer|seller 1 & 2 have sub-optimal strategies as they are exposed to the full amount of their credit link with reference entity 1.

We find that, such a configuration could be a possible candidate for modelling dependencies in the CDS market; however, such a construction represents a set of sub-optimal strategies of the market participants. For instance, $Buyer3$, would benefit from diversifying its risk arising from the fragility of $(Buyer|Seller)_1$.

### 3.3 Buyers-Sellers-Reference non-separable

In this set of configurations we impose that the intersection of buyers, sellers and reference entities is non-trivial.

Due to the level of complexity, we assign a label to each of the solid arrows to reflect the reference entity that is involved in a particular CDS contract. Consider figure 4, we keep the same convention as before. $(Buyer|Seller|Reference)_1$ buys CDS from $(Buyer|Seller|Reference)_2$ due to its pre-existing relationship with $(Buyer|Seller|Reference)_3$. $(Buyer|Seller|Reference)_2$ buys a CDS contract from $(Buyer|Seller|Reference)_3$ on a reference entity $(Buyer|Seller|Reference)_4$. In this scenario, if $(Buyer|Seller|Reference)_3$ defaults, $(Buyer|Seller|Reference)_1$ experiences an increase in fragility, due to its pre-existing relationship with $(Buyer|Seller|Reference)_3$ . In addition, $(Buyer|Seller|Reference)_1$ partly covers his losses due to a long CDS on $(Buyer|Seller|Reference)_3$ from $(Buyer|Seller|Reference)_2$. In turn, $(Buyer|Seller|Reference)_2$ on one hand looses from selling a CDS contract to $(Buyer|Seller|Reference)_1$, and at the same time experiences a greater exposure to $(Buyer|Seller|Reference)_4$. In addition, the health of $(Buyer|Seller|Reference)_3$ is dependent on $(Buyer|Seller|Reference)_4$, thus in case of a default of $(Buyer|Seller|Reference)_4$ can lead to an increase of fragility of $(Buyer|Seller|Reference)_3$, which in-turn affects both $(Buyer|Seller|Reference)_1$ and $(Buyer|Seller|Reference)_2$.

**Scenario 1: Figure 5 -** $(Buyer|Seller|Reference)_4$ **defaults**
In this scenario we assume that all the market participants play all three roles:

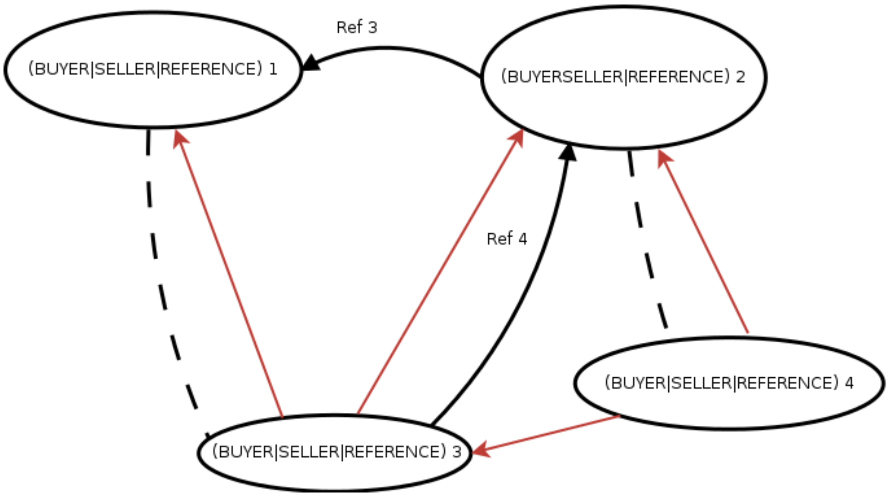


Figure 4: **Networks that might exist when the buyers, sellers and reference entities are non-separable**. The solid arrow moves from the seller of a CDS contract to the buyer. The dotted arrow refers to the reference entity underlying the CDS contract. Solid lines are labeled with the reference entity that is involved in a CDS contract. The red arrows represent the direction of impact in the event of a default of the node from which the arrow emerges

buyer, seller, and reference entity. Suppose that $(Buyer|Seller|Reference)_4$ defaults, then $(Buyer|Seller|Reference)_3$, $(Buyer|Seller|Reference)_1$, and $(Buyer|Seller|Reference)_2$ are all affected. $(Buyer|Seller|Reference)_2$ suffers a marginal loss on account of a CDS bought from $(Buyer|Seller|Reference)_3$. However, large percentage of $(Buyer|Seller|Reference)_4$ loss is transferred to $(Buyer|Seller|Reference)_3$, which in turn makes $(Buyer|Seller|Reference)_2$ more fragile as $(Buyer|Seller|Reference)_3$'s fragility makes $(Buyer|Seller|Reference)_2$ more liable to make a payment to $(Buyer|Seller|Reference)_1$. Thus, we see that the default of $(Buyer|Seller|Reference)_4$, which seems rather disconnected from a trading perspective, can in-fact affect the fragility of $(Buyer|Seller|Reference)_1$, that does not have a direct relationship with $(Buyer|Seller|Reference)_4$. Thus, we see that in case: if buyers, sellers and reference entities can be either or all, in that case the system can experience co-movements reflecting interconnections that are otherwise non-explicit.

**Scenario 2: Figure 5 -** $(Buyer|Seller|Reference)_4$ **defaults**

In the event that $(Buyer|Seller|Reference)_4$ defaults, it would make $(Buyer|Seller|Reference)_2$, and $(Buyer|Seller|Reference)_3$ more fragile. $(Buyer|Seller|Reference)_2$ could recover most of its losses from the default of $(Buyer|Seller|Reference)_4$ due to its purchase of a CDS contract on

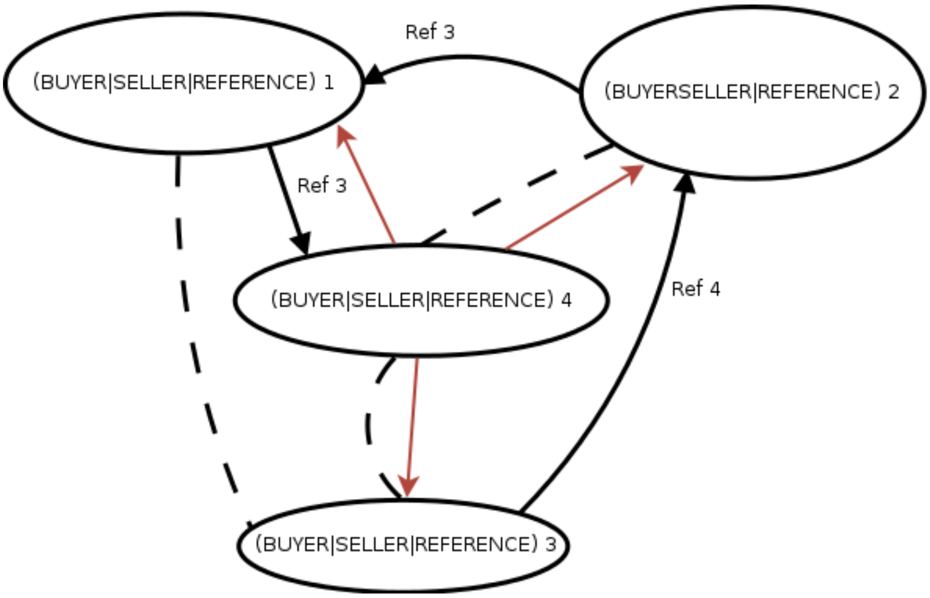


Figure 5: **Networks that exist when the buyers and sellers are the same but different from reference entities**. The solid arrow moves from the seller of a CDS contract to the buyer. The dotted arrow refers to the reference entity underlying the CDS contract. The red arrows represent the direction of impact in the event of a default of the node from which the arrow emerges

$(Buyer|Seller|Reference)_3$. $(Buyer|Seller|Reference)_3$ experiences fragility due to the default of $(Buyer|Seller|Reference)_4$. The increased fragility of $(Buyer|Seller|Reference)_3$, makes $(Buyer|Seller|Reference)_1$ more fragile as it is the seller of protection on $(Buyer|Seller|Reference)_3$ to $(Buyer|Seller|Reference)_4$. In turn the fragility of $(Buyer|Seller|Reference)_1$ might adversely affect $(Buyer|Seller|Reference)_4$ if it would not be in a position to fulfil its obligations to $(Buyer|Seller|Reference)_4$.

We see here that there is a feedback loop that emerges from the distress of $(Buyer|Seller|Reference)_4$ to itself. In addition,

**Scenario 3: Figure 6 -** $(Buyer|Seller|Reference)_3$ **defaults**

In the event that $(Buyer|Seller|Reference)_3$ defaults, it affects $(Buyer|Seller|Reference)_2$, $(Buyer|Seller|Reference)_1$, and $(Buyer|Seller|Reference)_4$. Default of $(Buyer|Seller|Reference)_3$ would imply that $(Buyer|Seller|Reference)_2$ would be liable to $(Buyer|Seller|Reference)_1$ for the majority of the loss. $(Buyer|Seller|Reference)_1$ would be marginally affected by the default of $(Buyer|Seller|Reference)_3$. However,

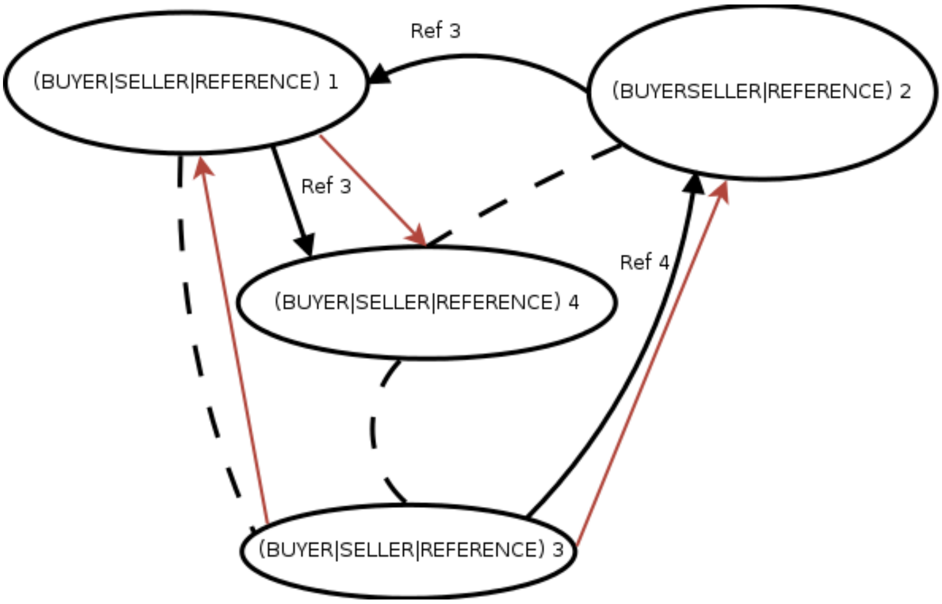


Figure 6: **Networks that exist when the buyers and sellers are the same but different from reference entities**. The solid arrow moves from the seller of a CDS contract to the buyer. The dotted arrow refers to the reference entity underlying the CDS contract.

$(Buyer|Seller|Reference)_1$ would experience a loss due to the fact that it has sold protection to $(Buyer|Seller|Reference)_4$. In the even that $(Buyer|Seller|Reference)_1$ defaults due to the default of $(Buyer|Seller|Reference)_3$, then $(Buyer|Seller|Reference)_4$ would be distressed due to the default of $(Buyer|Seller|Reference)_3$.

We find that when we impose the intersection of the set of buyers, sellers and reference entities to be non-trivial. Then, we observe a dependence structure that would introduce *interdependence* in the time series of the market participants. With this framework, where the buyers and sellers for each CDS contract are unknown, we can still model dependencies among financial entities utilising their CDS time series data.

## 4 Correlation analysis

There are many financial entities that are already intertwined with each other based on ownerships and mergers, among others. Thus, it is possible to expect that the price evolution of the CDS spread of subsidiary of a parent company would, in some sense, mimic the behaviour of the CDS spread of its parent entity. It is possible that the evolution of the time series of subsidiary of a firm and its parent entity have a correlation coefficient of zero; however, we know that in the

case of correlation analysis a correlation coefficient of 0 does not imply independence. Thus, one may not assume that the time series of a time series of a parent company and its subsidiary are independent; but, one can certainly not extract the underlying ownership relationship embedded in the time series of the two. Thus we find that performing the analysis of dependence structures via the method of correlation analysis might not be the most appropriate choice in this case. We proceed to make some observations on a traditional measure of dependence in order to highlight the reasoning for pursuing a $\varepsilon$-drawup co-movement framework.

Correlation analysis presents some pitfalls that mask the underlying dependence structure. If two random variables are independent, then they imply that they are uncorrelated; however, a correlation of zero does not imply that two random variables are independent. Suppose we have two jointly distributed real valued random variables. The linear coefficient of correlation is $\rho(X, Y)$ is defined as

$$\rho(X, Y) = \frac{E[(X - \mu_X)(Y - \mu_Y)]}{\sigma_X \sigma_Y} \tag{1}$$

In addition, if the variances of random variables are not finite, then linear correlation is not defined for such a pair (McNeil et al., 2005).

. To this end, we deviate from a using correlation analysis to explain dependence among financial firms.

# 5 Remarks on Drawup Detection

CDS time series data were polished beforehand to make the analysis in the $\varepsilon$-drawups framework possible. Not all time series exist in the same time window, thus we take the CDS contract with the largest number of observations and use it as a reference of our time window. Thus, all time series are put in one matrix, where if a CDS time series did not exist whence the reference existed, then we assign a value of zero to it. This modification does not affect the dynamics of the CDS's per se, as a spread of zero implies an absence of a swap contract anyways. Once, we have the data in a single matrix, we then iterate through all the individual time series and compute all the local extrema (see Methods in the main paper). The date of each extrema is also recorded. We then proceed to computing $\varepsilon$-drawups. The $\varepsilon$ parameter is a local and dynamic parameter. It is essentially the local variation of a time series in the last ten days. We compute the $\varepsilon$-drawups for each security and record the date at which the $\varepsilon$-drawup occurred. We then proceed to computing co-drawups pairwise. To compute common drawups we divide the dataset into three periods (see Methods in the main paper) and compute common drawups and the drawups experienced by each of the time series in that period. We also compute co-drawups for all the pairs with a time delay factor $\tau$, i.e., when one security is translated by $\tau$ days w.r.t. another. We do this exercise for all pairs in our dataset. Finally, we compute $w_{ij}$'s (as before) using our count matrices.

# 6 Control Set

After having computed a matrix of $\varepsilon$-drawup's, for each security, we permute the matrix indices of where the $\varepsilon$-drawup's occur. This way we are re-arranging all the occurrences of $\varepsilon$-drawup's in a random manner. The reason to pursue this methodology and not generating random (or even , trend reinforced random walks) is that the authors don't wish to define the the price process as a priori, assuming random walks (or, trend reinforced random walks) are a good proxy for a CDS price process. In addition, we do not resample the original time series, as such a procedure introduces price movements that sometimes amplify $\varepsilon$-drawup's when there in fact are none. This key point becomes even more important when we want to develop a control set for all three periods. We perform a permutation test to filter the empirical $W'_{ij}s$. We compute $W'_{ij}$ for each pairs of securities. To do this, we proceed with permuting the $\varepsilon$-drawups in each of the securities and compute $W'_{ij}$. We repeat this procedure a hundred times. With the hundred realisations of $W'_{ij}$ for each pair of securities $i, j$, we then further filter $W'_{ij}$ at the 95% confidence interval to derive a single number $W^*_{ij}$ for each pair of securities. We then utilise $W^*_{ij}$ as the control number to filter empirical $W_{ij}$, i.e., each empirical pair is filtered with a unique number that corresponds to the control number generated from our permutation test.

# 7 PageRank and impact centrality

To compute the centrality of the nodes in the network, we take inspiration from the concept of PageRank that was introduced in the context of the World Wide Web (WWW) to enhance users' search experience (Page et al., 1998). The main theme of the idea revolved around determining the rank of a webpage based upon how many sites (other than itself) point towards it. Such a rank could be used as a good proxy for determining a webpages' relevance to user searches. Suppose, that the PageRank of each website, $i$, be denoted as $C_i$. Then, $C_i$ for websites can be defined in a network framework consisting of $N$ vertices. Consider,

$$C_i = \underbrace{\alpha \sum_{j \to i} \frac{C_j}{k^o_j}}_{\text{term 1}} + \underbrace{(1-\alpha)\frac{1}{N}}_{\text{term 2}} . \tag{2}$$

The $\alpha$ in term 1 on the r.h.s. of equation 2 represents the probability of $C_j$ inherited by webpages $j$ that are pointing to webpages $i$. Each webpage $j$ contributes, proportionally $\frac{C_j}{k^o_j}$, to the webpage it points points to. Term 2 in 2 uniformly assigns the contribution of each of the webpages $j$ to $i$ times the complimentary probability from term 1. Unlike our measure of centrality, i.e., impacted-impacting centrality, PageRank centrality measure is row stochastic. Impacted-impacting centrality is analogous to the cumulative distress in the network on account of distress in node $i$.

## 8 The Bow-tie Structure & FCIC Report

**A bowtie structure** refers to a directed graph here, where the connected nodes are in one of the three parts of the network: IN (nodes with outgoing links only), SCC (nodes with both incoming and outgoing links) and OUT (nodes with incoming links). The resulting structure resembles that of a bow-tie where the SCC occupies the position of a knot and the IN and OUT represent the respective wings of the tie. It is important to remember that the bow-tie structure is a construction that largely depends on the thresholds that are imposed upon the impacting-impacted centrality. We present the bow-tie structures from periods 1 until 3. The nodes are in the IN, if $r_i > 3/2$, see figures 7, 8, & 9. The nodes in the SCC have $2/3 < r_i < 3/2$, and nodes are in the OUT, if $r_i < 2/3$. We also present the distributions of in-degree, out-degree, impacting, and impacted centralities for all three periods. We find that even though in-degree and out-degree have mass of their distributions in a narrow range; the impacting and impacted centralities across the three periods are distributed across a wider spectrum. Additionally, we present bow-tie structures from all three periods with varying degrees of thresholding, see figures 12, 13, 14, 15, 16, 17, and 11. The existence of the bow-tie structure is not guaranteed in all graphs. Consider, figures 10a) & b). With these counterexamples we highlight that the existence of a bow-tie structure is not assured after the separation of nodes based on their level of impacting-impacted centrality. We find that in our network there is an SCC in all three periods after filtering the impacting-impacted centrality.

**The Financial Crisis Inquiry Commission** (FCIC) was established under the Fraud Enforcement and Recovery Act (Public Law 111-21) and was later passed by the Congress and officially signed and implemented by the President of the US in the month of May, 2009.

The goals of the FCIC was to examine the causes that led to the financial and economic crisis of 2008. During their investigation the FCIC conducted more that 700 witnesses and reviewed millions of documents. In addition, it also held public hearings in New York, Washington D.C. among other regions in the US. FCIC conducted extensive case studies on firms that it deemed as pivotal in bringing about the crisis. These firms include: American International Group (AIG), Bear Stearns, Citigroup, Countrywide Financial, Fannie Mae, Goldman Sachs, Lehman Brothers, Merrill Lynch, Moody's and Wachovia.

We present brief snapshots from the FCIC report FCIC (2011) of some of the firms that the FCIC indicated were pivotal in financial crisis of 2008 along with the bow-tie visualisations from each of the three periods, see fig. 1. In addition we also present the degree distributions for all three periods. We also present some statistics on the distributions of nodes in the various regions of the *bow-tie* structure, see table 1, and the movement of some pivotal firms across the *bow-tie* structure in the three periods, see table 2.

**AIG**:

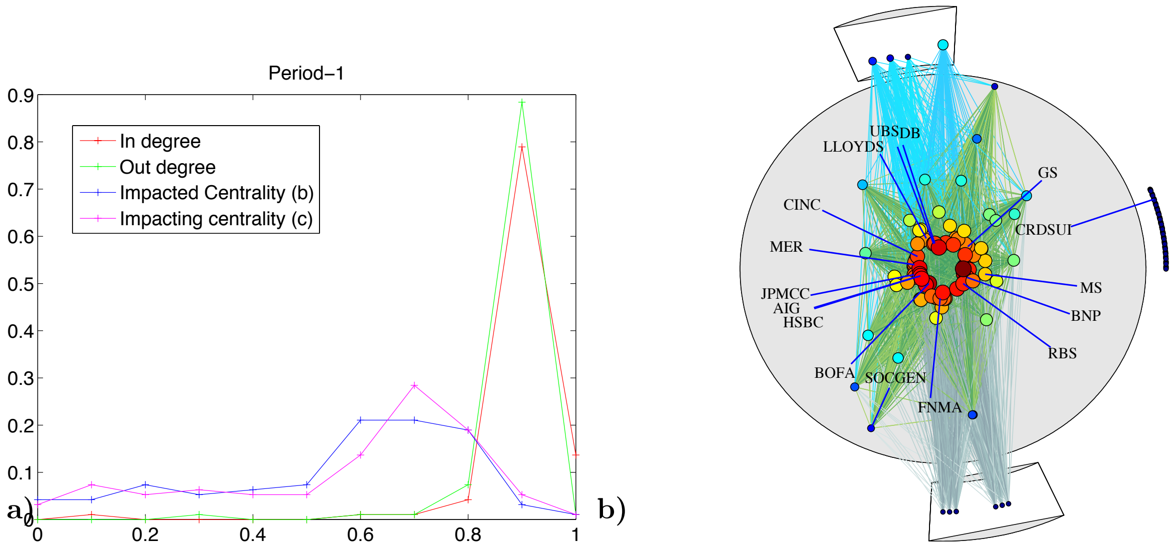


Figure 7: **a) The normalised distribution of in-degree, out-degree, impacting and impacted centralities in period 1** . The bulk of the in-degree and out-degree distributions are concentrated in a narrow range. Impacted and impacted centrality distributions are distributed across the x-axis. **b) The network of the CDS reference entities from period 1**. Each of the nodes represents a financial institution. Outgoing links from nodes that are in the top, or the IN of the bow-tie structure represent the estimated potential impact of a financial institution to its neighbours (see Methods). The nodes in the SCC are placed within a circle of radius one and centred at the origin. The distance of each node from the centre is 1−Impacting centrality. The angle increases linearly from 0 to $2\pi$. Thus, the closer a node is to the centre the higher is impacted-impacting centrality. Similarly, nodes in the OUT and IN are placed between angles $\pi/2$- $5\pi/8$ and $3\pi/2$ - $13\pi/8$ respectively. In addition, nodes in the OUT and IN are placed with an offset of 1.1 from the origin. With the bow-tie representation we are able to visually compare the centrality of a node $i$ with node$j$. Also, with this visualisation we are able to extract a network of nodes that mostly impact the others, nodes that impact just as much as they get impacted, and nodes that only get impacted by other nodes in the network. The size and the colour of the node reflects impacted-impacting centrality of a node (nodes with larger impacted-impacting centrality are in red). The colour assigned to links is based on where the links point to in the network. Links originating from IN to the SCC are in bright blue. Links originating in the SCC to nodes in the SCC are in green. Links that are originating in the SCC to the OUT are dull blue grey colour.

- By 2005, AIG had written $107 billion in CDS for such regulatory capital benefits; most were with European banks for a variety of asset types. That total would rise to $379 billion

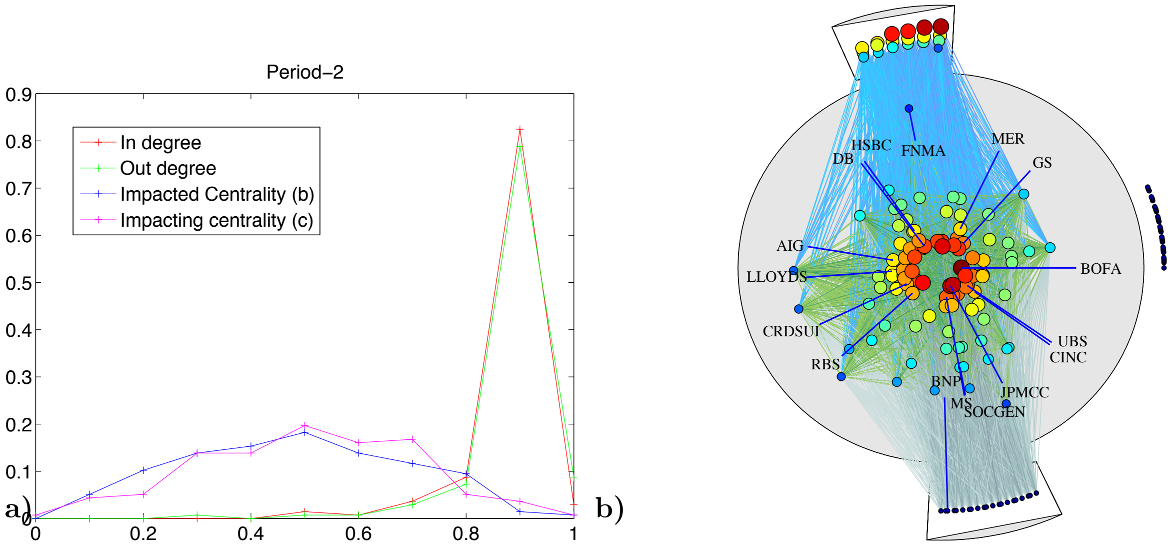


Figure 8: **a) The normalised distribution of in-degree, out-degree, impacting and impacted centralities in period 2** . The bulk of the in-degree and out-degree distributions are concentrated in a narrow range. Impacted and impacted centrality distributions are distributed across the x-axis. **b)The network of the CDS reference entities from period 2**. The bow-tie is constructed as described in fig. 7.

| | Impacting | Impacted | Both |
|---|---|---|---|
| Period 1 | 6 | 4 | 85 |
| Period 2 | 22 | 19 | 97 |
| Period 3 | 53 | 37 | 47 |

Table 1: Breakdown of nodes by region

by 2007. The same advantages could be enjoyed by banks in the United States, where regulators had introduced similar capital standards for banks' holdings of mortgage-backed securities and other investments under the Recourse Rule in 2001. So a credit default swap with AIG could also lower American banks' capital requirements. In 2004 and 2005, AIG sold protection on super-senior CDO tranches valued at $54 billion, up from just $2 billion in 2003. *FCIC Report*, page 140.

- AIG's business of offering credit protection on assets of many sorts, including mortgage-backed securities and CDOs, grew from $20 billion in 2002 to $211 billion in 2005 and $533 billion in 2007, *FCIC Report*, page 141.

**GS**

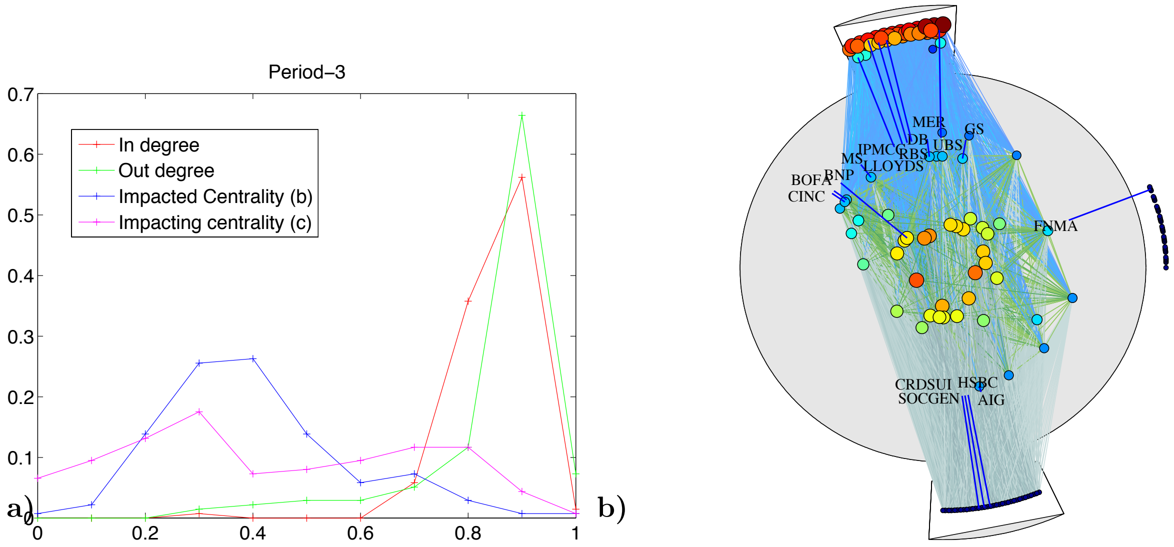


Figure 9: **a) The normalised distribution of in-degree, out-degree, impacting and impacted centralities in period 3** . The bulk of the in-degree and out-degree distributions are concentrated in a narrow range. Impacted and impacted centrality distributions are distributed across the x-axis. Unlike periods 1 & 2, the in-degree and out-degree distributions are less peaked. **b)The network of the CDS reference entities from period 3**. The bow-tie is constructed as described in fig. 7.

| | Period 1 | Period 2 | Period 3 |
|---|---|---|---|
| AIG | SCC | SCC | OUT |
| GS | SCC | SCC | SCC (periphery) |
| BOFA | SCC | SCC | SCC (periphery) |
| CINC | SCC | SCC | SCC (periphery) |
| JPMCC | SCC | SCC | IN |

Table 2: Location of AIG, GS, BOFA, CINC & JPMCC across the three periods in the *bow-tie* structure

- Second, CDS were essential to the creation of synthetic CDOs. These synthetic CDOs were merely bets on the performance of real mortgage-related securities. They amplified the losses from the collapse of the housing bubble by allowing multiple bets on the same securities and helped spread them throughout the financial system. Goldman Sachs alone packaged and sold \$73 billion in synthetic CDOs from July 1, 2004, to May 31, 2007. Synthetic CDOs created by Goldman referenced more than 3,400 mortgage securities, and 610 of them were referenced at least twice. This is apart from how many times these

securities may have been referenced in synthetic CDOs created by other firms. *FCIC Report*, Conclusions.

- Goldman Sachs estimated that between 25% and 35% of its revenues from 2006 through 2009 were generated by derivatives, including 70% to 75% of the firm's commodities business, and half or more of its interest rate and currencies business. From May 2007 through November 2008, $133 billion, or 86%, of the $155 billion of trades made by Goldman's mortgage department were derivative transactions. *FCIC Report*, pages 51-52.

- Goldman's assets grew from $250 billion in 1999 to $1.1 trillion by 2007, an annual growth rate of 21%, *FCIC Report*, page 65.

### BOFA, CINC, JPMCC

- From 1998 to 2007, the combined assets of the five largest U.S. banks: Bank of America, Citigroup, JP Morgan, Wachovia, and Wells Fargo more than tripled, from $2.2 trillion to $6.8 trillion.

- Leverage: Bank of America's leverage rose from 18:1 in 2000 to 27:1 in 2007. Citigroup's leverage increased from 18:1 to 22:1, then shot up to 32:1 by the end of 2007. *FCIC Report*, page 65.

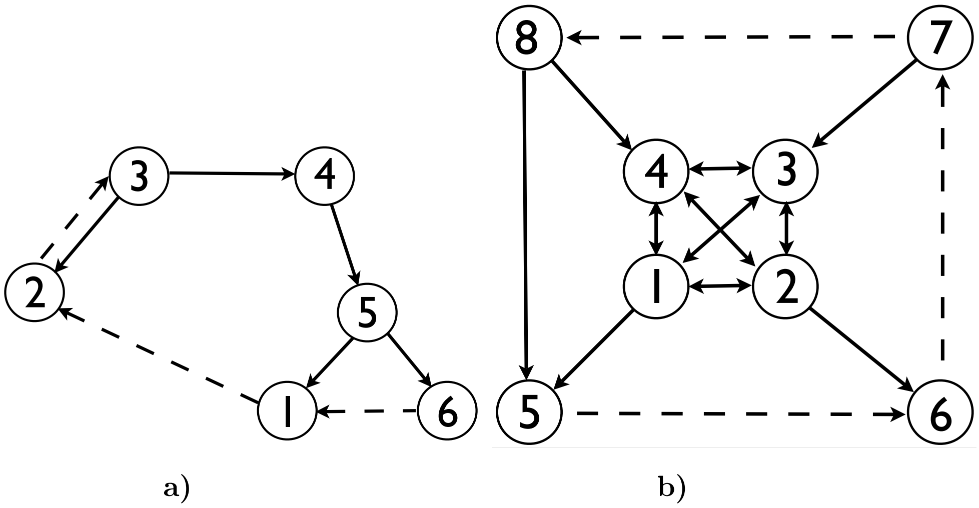


Figure 10: **a) Network $W$ with an SCC:** Dashed links are links that have been removed on the condition that $r_i < \theta$, where $\theta$ is some threshold. Then, we see that $W$ no longer consists an SCC. **b) Network $W$ with an SCC:** Dashed lines are as in **a)**. Then we see that, $W$ still has an SCC. In fact nodes 1,2,3, and 4 remain in the SCC (as before) even after filtering links.

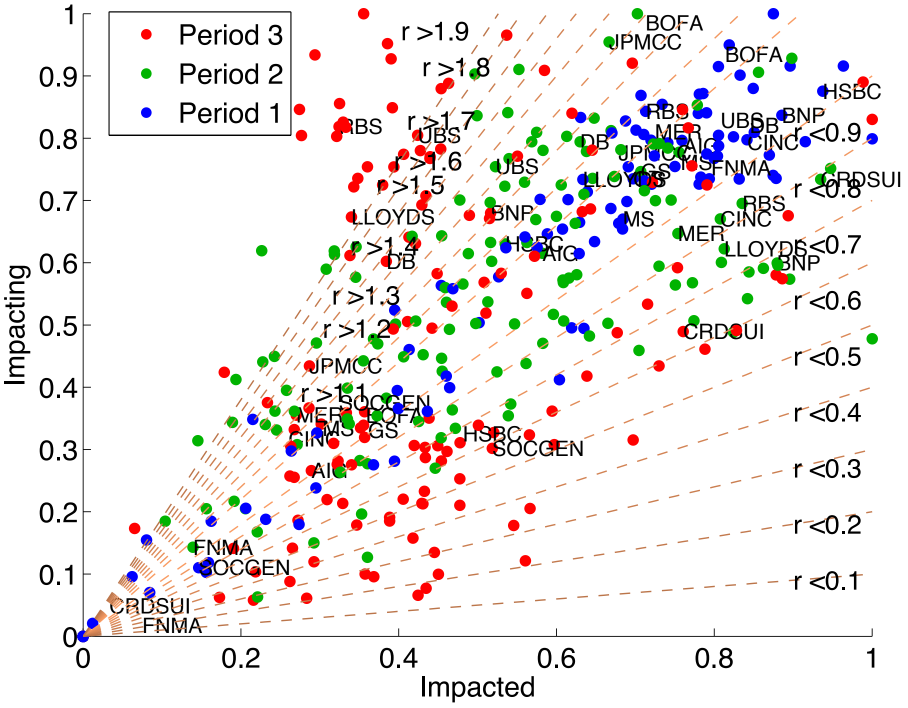


Figure 11: **Scatter plot of impacting versus impacted centrality**. Each institution in the CDS market is represented by three dots depending on the period (blue, green, red refers to period 1, 2, 3, respectively). It can be seen that, while in period 1 most institutions are located between the two dotted lines, in period 2 and 3 many of them move to the top and bottom region. This means that ratio between the two centrality measures varies with the market phase. Few institutions of interest are labelled. For example, Bank of America (BOFA) remains in the same region across the three periods. With reference to the subsequent bow-tie construction used in Figures 12, 13, 14, 15, 16, 17, and 11: The scatter plot is divided into 3 regions for each choice of $\delta \in \{0.1, 0.2, 0.3, 0.4, 0.5, 0.6, 0.7, 0.8, 0.9\}$ where the upper and lower regions are given by $1+\delta$, and $1-\delta$ respectively. Nodes in the region above the line $r_i > 1+\delta$ correspond to the IN. Nodes in the region $1-\delta < r_i < 1+\delta$ correspond to the SCC. Nodes in the region $r_i < 1-\delta$ correspond to the OUT.

## Acknowledgments

The authors acknowledge the financial support from the Swiss National Science Foundation Grant CR12I1-127000) and the European Commission FET Open Project “FOC” 255987.

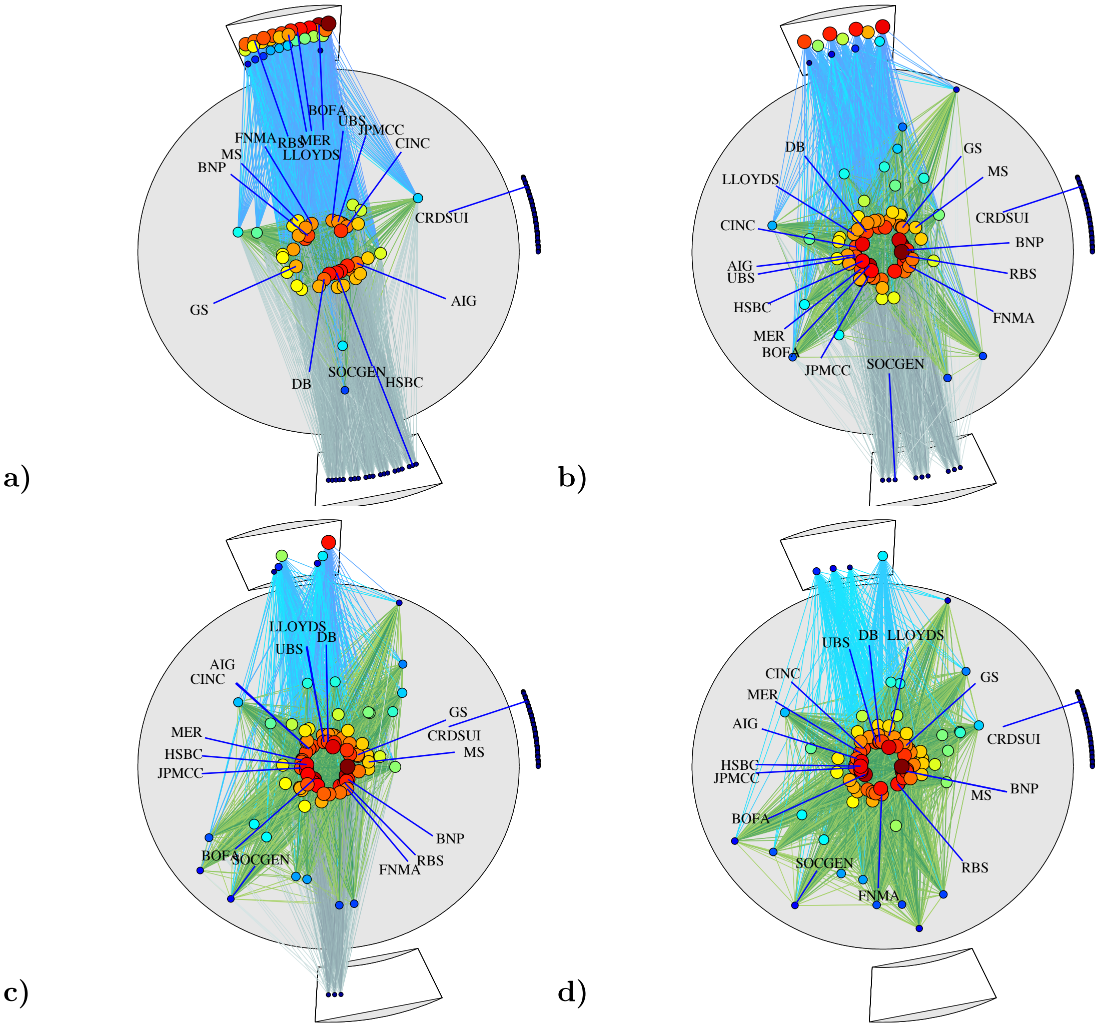


Figure 12: **Bow-tie structure from period 1 for varying values of impacting-impacted centralities a)** The bow-tie is constructed as in figure 7. Nodes with $0.9 < r_i < 1.1$ are in the SCC, nodes with $r_i > 1.1$ are in the IN, and the nodes with $r_i < 0.9$ are in the OUT **b)** The bow-tie is constructed as in figure 7. Nodes with $0.8 < r_i < 1.2$ are in the SCC, nodes with $r_i > 1.2$ are in the IN, and the nodes with $r_i < 0.8$ are in the OUT **c)** The bow-tie is constructed as in figure 7. Nodes with $0.7 < r_i < 1.3$ are in the SCC, nodes with $r_i > 1.3$ are in the IN, and the nodes with $r_i < 0.7$ are in the OUT **d)** The bow-tie is constructed as in figure 7. Nodes with $0.7 < r_i < 1.3$ are in the SCC, nodes with $r_i > 1.3$ are in the IN, and the nodes with $r_i < 0.7$ are in the OUT

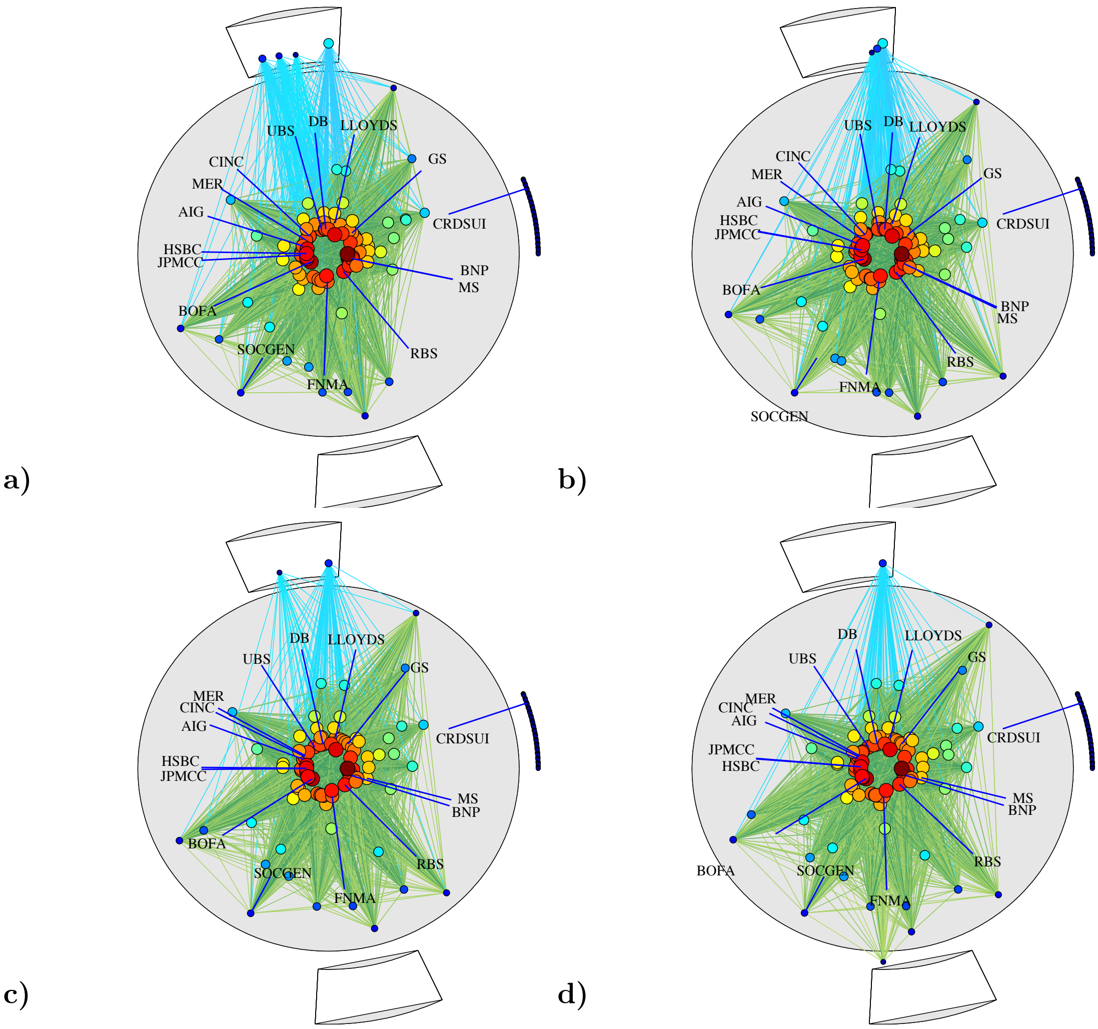


Figure 13: **Bow-tie structure from period 1 for varying values of impacting-impacted centralities a)** The bow-tie is constructed as in figure 7. Nodes with $0.5 < r_i < 1.5$ are in the SCC, nodes with $r_i > 1.5$ are in the IN, and the nodes with $r_i < 0.5$ are in the OUT **b)** The bow-tie is constructed as in figure 7. Nodes with $0.4 < r_i < 1.6$ are in the SCC, nodes with $r_i > 1.6$ are in the IN, and the nodes with $r_i < 0.4$ are in the OUT **c)** The bow-tie is constructed as in figure 7. Nodes with $0.3 < r_i < 1.7$ are in the SCC, nodes with $r_i > 1.7$ are in the IN, and the nodes with $r_i < 0.3$ are in the OUT **d)** The bow-tie is constructed as in figure 7. Nodes with $0.2 < r_i < 1.8$ are in the SCC, nodes with $r_i > 1.8$ are in the IN, and the nodes with $r_i < 0.2$ are in the OUT

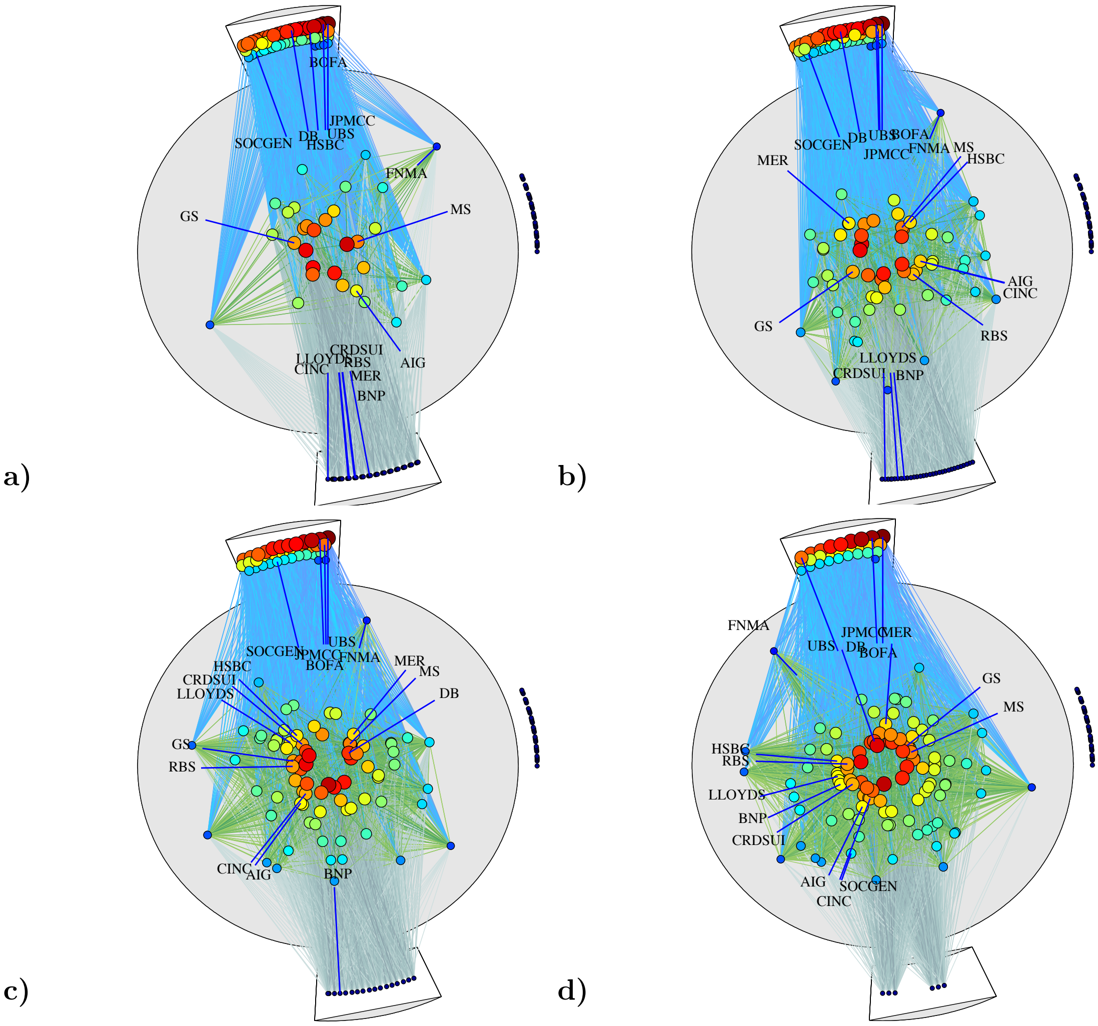


Figure 14: **Bow-tie structure from period 2 for varying values of impacting-impacted centralities a)** The bow-tie is constructed as in figure 7. Nodes with $0.9 < r_i < 1.1$ are in the SCC, nodes with $r_i > 1.1$ are in the IN, and the nodes with $r_i < 0.9$ are in the OUT **b)** The bow-tie is constructed as in figure 7. Nodes with $0.8 < r_i < 1.2$ are in the SCC, nodes with $r_i > 1.2$ are in the IN, and the nodes with $r_i < 0.8$ are in the OUT **c)** The bow-tie is constructed as in figure 7. Nodes with $0.7 < r_i < 1.3$ are in the SCC, nodes with $r_i > 1.3$ are in the IN, and the nodes with $r_i < 0.7$ are in the OUT **d)** The bow-tie is constructed as in figure 7. Nodes with $0.7 < r_i < 1.3$ are in the SCC, nodes with $r_i > 1.3$ are in the IN, and the nodes with $r_i < 0.7$ are in the OUT

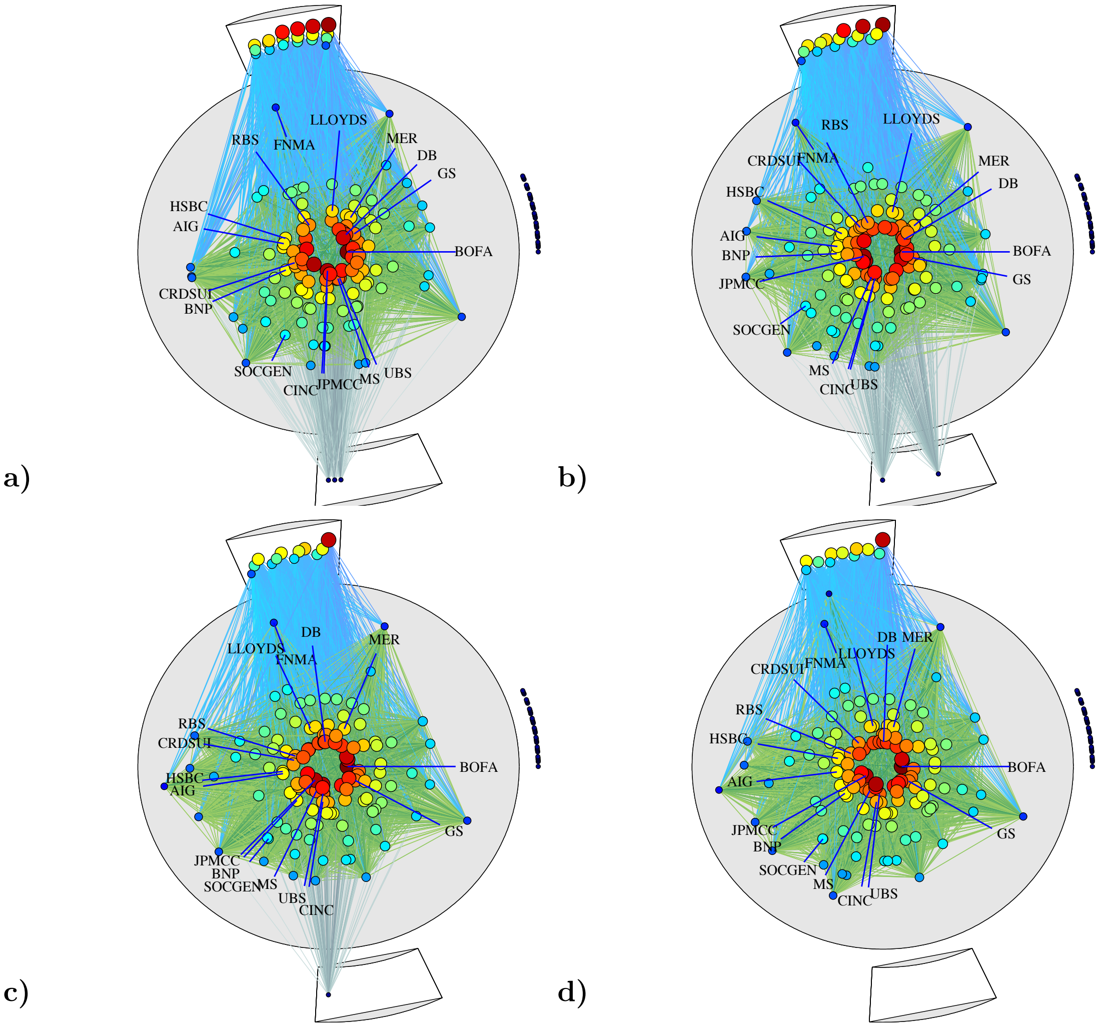


Figure 15: **Bow-tie structure from period 2 for varying values of impacting-impacted centralities a)** The bow-tie is constructed as in figure 7. Nodes with $0.5 < r_i < 1.5$ are in the SCC, nodes with $r_i > 1.5$ are in the IN, and the nodes with $r_i < 0.5$ are in the OUT **b)** The bow-tie is constructed as in figure 7. Nodes with $0.4 < r_i < 1.6$ are in the SCC, nodes with $r_i > 1.6$ are in the IN, and the nodes with $r_i < 0.4$ are in the OUT **c)** The bow-tie is constructed as in figure 7. Nodes with $0.3 < r_i < 1.7$ are in the SCC, nodes with $r_i > 1.7$ are in the IN, and the nodes with $r_i < 0.3$ are in the OUT **d)** The bow-tie is constructed as in figure 7. Nodes with $0.2 < r_i < 1.8$ are in the SCC, nodes with $r_i > 1.8$ are in the IN, and the nodes with $r_i < 0.2$ are in the OUT

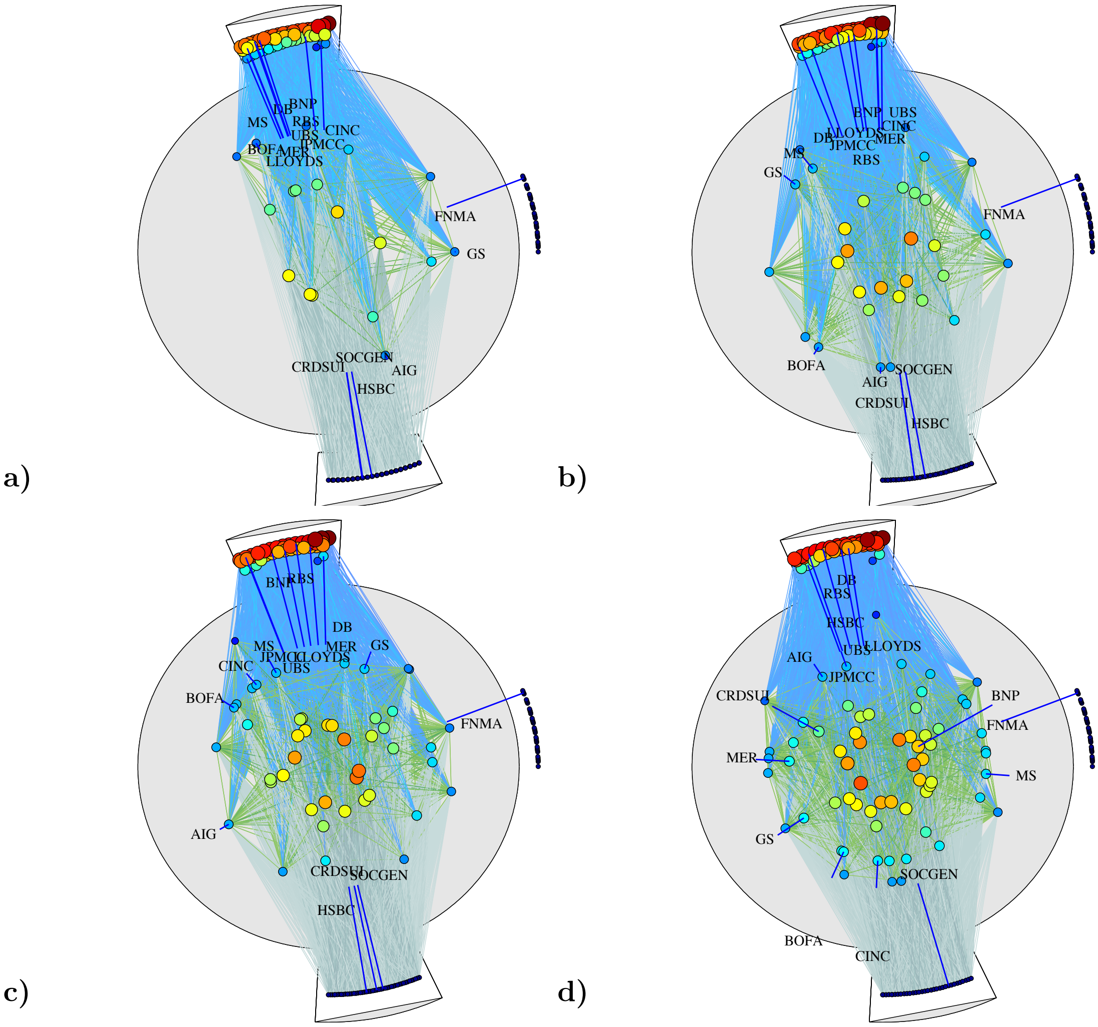


Figure 16: **Bow-tie structure from period 3 for varying values of impacting-impacted centralities a)** The bow-tie is constructed as in figure 7. Nodes with $0.9 < r_i < 1.1$ are in the SCC, nodes with $r_i > 1.1$ are in the IN, and the nodes with $r_i < 0.9$ are in the OUT **b)** The bow-tie is constructed as in figure 7. Nodes with $0.8 < r_i < 1.2$ are in the SCC, nodes with $r_i > 1.2$ are in the IN, and the nodes with $r_i < 0.8$ are in the OUT **c)** The bow-tie is constructed as in figure 7. Nodes with $0.7 < r_i < 1.3$ are in the SCC, nodes with $r_i > 1.3$ are in the IN, and the nodes with $r_i < 0.7$ are in the OUT **d)** The bow-tie is constructed as in figure 7. Nodes with $0.7 < r_i < 1.3$ are in the SCC, nodes with $r_i > 1.3$ are in the IN, and the nodes with $r_i < 0.7$ are in the OUT

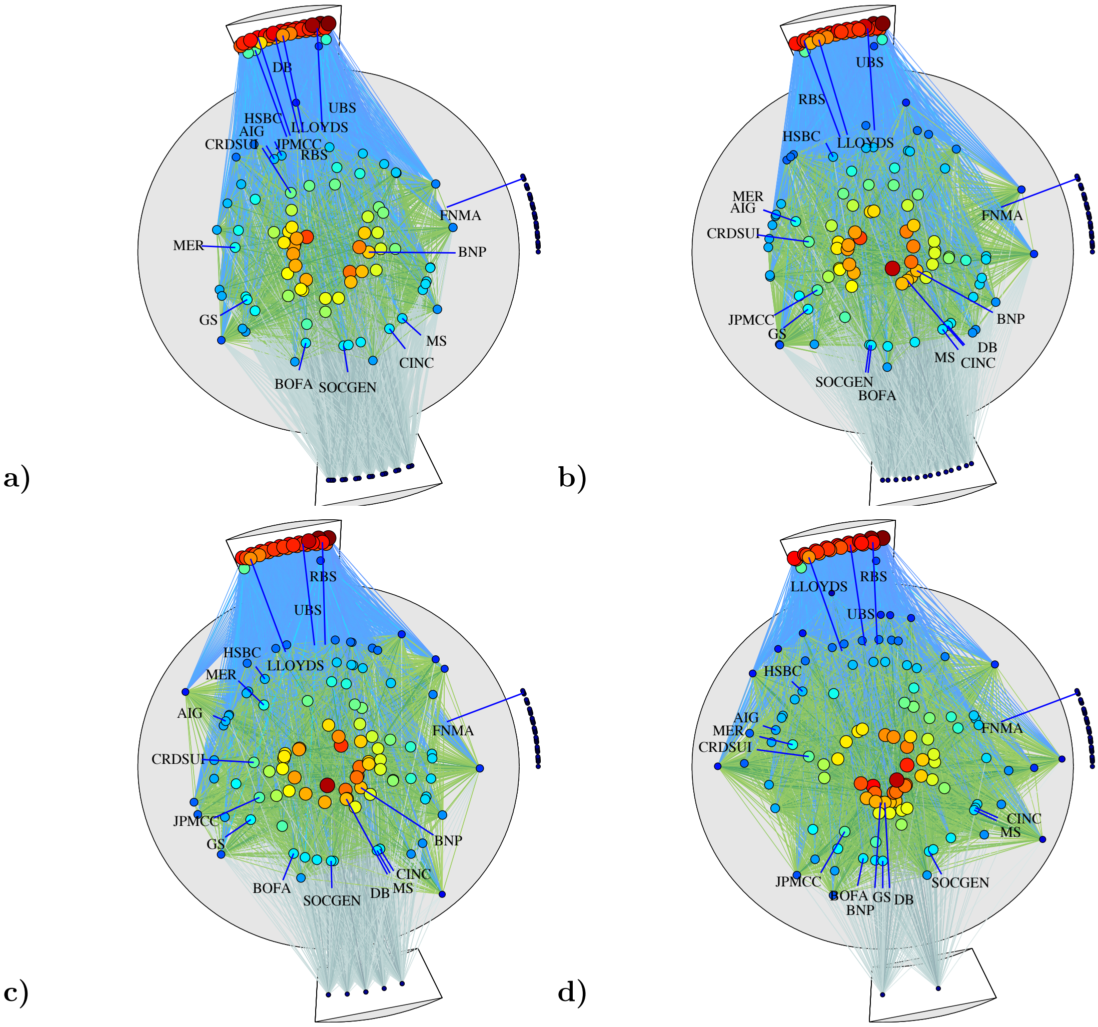


Figure 17: **Bow-tie structure from period 3 for varying values of impacting-impacted centralities a)** The bow-tie is constructed as in figure 7. Nodes with $0.5 < r_i < 1.5$ are in the SCC, nodes with $r_i > 1.5$ are in the IN, and the nodes with $r_i < 0.5$ are in the OUT **b)** The bow-tie is constructed as in figure 7. Nodes with $0.4 < r_i < 1.6$ are in the SCC, nodes with $r_i > 1.6$ are in the IN, and the nodes with $r_i < 0.4$ are in the OUT **c)** The bow-tie is constructed as in figure 7. Nodes with $0.3 < r_i < 1.7$ are in the SCC, nodes with $r_i > 1.7$ are in the IN, and the nodes with $r_i < 0.3$ are in the OUT **d)** The bow-tie is constructed as in figure 7. Nodes with $0.2 < r_i < 1.8$ are in the SCC, nodes with $r_i > 1.8$ are in the IN, and the nodes with $r_i < 0.2$ are in the OUT

# References

Battiston, S., Glattfelder, J. B., Garlaschelli, D., Lillo, F., and Caldarelli, G. (2010). The Structure of Financial Networks. *Network Science*, pages 131–163.

FCIC, F. C. I. C. (2011). *The financial crisis inquiry report: final report of the National Commission on the Causes of the Financial and Economic Crisis in the United States*. Public Affairs.

McNeil, A., Frey, R., and Embrechts, P. (2005). *Quantitative risk management: Concepts, techniques and tools*. Princeton Univ Pr.

Page, L., Brin, S., Motwani, R., and Winograd, T. (1998). The PageRank citation ranking: Bringing order to the web. Technical report, Stanford Digital Library Technologies Project.
